# Supplementary material for: Big Data of Materials Science - Critical Role of the Descriptor
Source: arXiv:1411.7437 ancillary file (2015-02-05)
Supplement: Supplementary file 1 [file Critical_Role_SI.pdf]

# BIG DATA OF MATERIALS SCIENCE – CRITICAL ROLE OF THE DESCRIPTOR: SUPPLEMENTARY INFORMATION

## 1. Details on the iterative LASSO-based approach for finding the best descriptor, applied to the 82 octet binary materials and $\Delta E = E(RS) - E(ZB)$ as property to be learned.

I) We start from atomic features (the column "#" indicates the number of features in the class described in the line):

| ID | Description | Symbols | # |
|---|---|---|---|
| $A1$ | Ionization Potential (IP) and Electron Affinity (EA) | IP(A) EA(A) IP(B) EA(B)[§] | 4 |
| $A2$ | Highest occupied (H) and lowest unoccupied (L) Kohn-Sham levels | H(A) L(A) H(B) L(B) | 4 |
| $A3$ | Radius at the max. value of $s$, $p$, and $d$ valence radial radial probability density | $r_s$(A) $r_p$(A) $r_d$(A) $r_s$(B) $r_p$(B) $r_d$(B) | 6 |

[§] We used for IP (EA) the energy of the half occupied Kohn-Sham orbital in the half positively (negatively) charged atom.

II) Our goal is to create physically well-formed combinations of the initial features. For example, we exclude linear combinations of inhomogeneous quantities, such as "IP + $r_s$" or "$r_s$ + $r_p^2$". Except the exclusions of physically unreasonable combinations, we produce as many combinations as possible. However, compressed sensing theory poses a limit on the maximum size $M$ of the feature space from which the best (low-) $\Omega$-dimensional descriptor can be extracted by sampling the feature space with the knowledge of $N$ data points : $N = A\Omega \ln(M)$ [1, 2, 3], when the $M$ candidate features are uncorrelated. $A$ is not a universal constant, however it is recommendable to have values between 4 and 8. For $\Omega = 2$ and $N = 82$, this implies a range of $M$ between $\sim 200$ and $\sim 30000$. Therefore, we regarded values of $M$ of few thousands as an upper limit of its size. Since the number of thinkable features is certainly larger than few thousands, we proceeded iteratively in several steps, by learning from the previous step what to put and what not in the candidate-feature list of the next step. In the next part of this section, we describe the final set of $\sim 4500$ features that we created for finding the actual descriptor as presented in the main text. Then, we summarize how we arrived at this particular set, i.e., the iterative procedure. First of all, we form sums and absolute differences of homogeneous quantities

| ID | description | prototype formula | # |
|---|---|---|---|
| $B1$ | absolute differences and sums of $A1$ | $\lvert\mathrm{IP(A)} \pm \mathrm{IP(B)}\rvert$ | 12 |
| $B2$ | absolute differences and sums of $A2$ | $\lvert\mathrm{L(B)} \pm \mathrm{H(A)}\rvert$ | 12 |
| $B3$ | absolute differences and sums of $A3$ | $\lvert r_p(\mathrm{A}) \pm r_s(\mathrm{A})\rvert$ | 30 |
| $C3$ | squares of $A3$ and $B3$ (only sums) | $r_s(\mathrm{A})^2, (r_p(\mathrm{A}) + r_s(\mathrm{A}))^2$ | 21 |
| $D3$ | exponentials of $A3$ and $B3$ (only sums) | $\exp(r_s(\mathrm{A})), \exp(r_p(\mathrm{A}) \pm r_s(\mathrm{A}))$ | 21 |
| $E3$ | exponentials of squared $A3$ and $B3$ (only sums) | $\exp(r_s(\mathrm{A})^2), \exp(r_p(\mathrm{A}) \pm r_s(\mathrm{A})^2)$ | 21 |

III) In turn, the above combinations are further combined:

| ID | description | prototype formula | # |
|---|---|---|---|
| $\{F1, F2, F3\}$ | Abs. differences and sums of $\{B1, B2, B3\}$, without repetitions | $\|r_p(\mathrm{A}) \pm r_s(\mathrm{A})\| + \|r_p(\mathrm{B}) \pm r_s(\mathrm{B})\|^\dagger$ | 72 |
| $X$ | ratios of any of $\{Ai, Bi\}, i = 1, 2, 3$ with any of $\{A3, C3, D3, E3\}$ | $\|r_p(\mathrm{B}) - r_s(\mathrm{B})\| / (r_d(\mathrm{A}) + r_s(\mathrm{B}))^3$ | $\sim 4300$ |

† With sign $-$, this is Zunger's $r_\pi$, with sign + Zunger's $r_\sigma$.

IV) LASSO is run in this set of $\sim$ 4500 candidate features. If the features were uncorrelated the first two features appearing when $\lambda$ is decreased would be the best 2D descriptor, i.e., the one that minimizes the RMSE. Correlation between pairs of features means in this context that the covariance (i.e., the scalar product of the 82-dimensional vectors containing the values of features $i$ and $j$, with each vector subtracted of its mean value and divided by its standard deviation) is close to 1 or -1. If their covariance is close to zero, the two features are uncorrelated.
Unfortunately, checking all pairs of features for covariance would scale with size $M$ as unfavorably as just performing the brute force search for the best 2D descriptor by trying all pairs. Furthermore, such a screening would require to define a threshold for the absolute value of the covariance for deciding whether any two features are correlated and possibly discarding one of the two. A similar problem would appear in case more refined techniques like singular value decomposition are tried in order to discard eigenvectors with low eigenvalues. Still a threshold should be defined and thus tuned.
We adopted instead a simple yet powerful solution: The best 30 features with non-zero coefficients that emerge at decreasing $\lambda$ are grouped, and among them an extensive test is performed: All single features, all pairs, all triples, ... are used as input for a linear least square fit. The single features, pairs, ... that score the lowest RMSE are the outcome of the procedure as 1D, 2D, ... descriptors. The validity of this approach (extensive test on 20-30 best candidates as selected by LASSO) was tested by running it on smaller feature spaces ($M \sim$ few hundreds) where the brute force all-pairs and all-triples search could be carried out.

In order to determine the final feature space as described above, we proceeded in this way:

- As scalar features describing the valence orbitals, we use the radii at which the radial probability densities of the valence $s$, $p$, ad $d$ orbitals have their maxima. This type of radii was in fact selected by our procedure, as opposed to the average radii (i.e., the quantum-mechanical expectation value of the radius). Namely, a feature space containing both sets of radii was constructed and only features containing the radii at maximum were selected among the best.
- Similarly, we also defined three other radius-derived features for the atoms: the radius of the highest occupied orbital of the neutral atom, $r_0$ (this is either $r_s$ or $r_p$ as defined above, but it generates over all the 82 compounds a set that is different from - and uncorrelated with - both $r_s$ and $r_p$), similarly defined radii for the anions, $r_-$, and the cations, $r_+$. As in the previous point, we constructed a feature space containing both $\{r_0, r_-, r_+\}$ and $\{r_s, r_p, r_d\}$ and their combinations, and found that only the latter radii were selected among the best.
- We have considered in addition features related to the AA, BB and AB dimers:

| ID | Description | Symbols | # |
|---|---|---|---|
| $A4$ | Binding energy | $E_b(\mathrm{AA})$ $E_b(\mathrm{BB})$ $E_b(\mathrm{AB})$ | 3 |
| $A5$ | HOMO-LUMO KS gap | HL(AA) HL(BB) HL(AB) | 3 |
| $A6$ | Equilibrium distance | $d(\mathrm{AA})$ $d(\mathrm{BB})$ $d(\mathrm{AB})$ | 3 |

These new features where combined in the same way as the classes $A1$, $A2$, and $A3$. After running our procedure, we find that features containing dimer-related quantities are never selected among the most prominent.

- We constructed in sequence several sets of features, in particular varying systematically the elements of class $X$. Multiplication of the $\{Ai, Bi, Ei\}$, $(i = 1, 2, 3)$ by the $\{A3, B3\}$ was included, as well as division of $\{Ai, Bi, Ei\}, (i = 1, 2, 3)$ by the $\{A3, B3\}$ cubed. Only division by $C3$ were selected by LASSO. At this stage, a descriptor in the form

$$\frac{|\mathrm{IP(B)} - \mathrm{EA(B)}|}{r_p(\mathrm{A})^2}, \frac{|r_s(\mathrm{A}) - r_p(\mathrm{B})|}{r_s(\mathrm{A})^2}, \frac{|r_p(\mathrm{B}) - r_s(\mathrm{B})|}{r_d(\mathrm{A})^2}$$

  was found.
  The persistence of the $C3$ class in the denominator suggested to try other decaying functions of $r$ and $r + r'$; for instance, exponentials as defined in $D3$ and $E3$. Interestingly, when the set of features containing $C3$, $D3$, and $E3$ was searched, the second and third component of the above descriptor were substituted by corresponding forms where the denominator squared is replaced by exponentials of the same atomic features (see below). This descriptor was therefore found by LASSO, in the sense that the substitutions $1/r_s(\mathrm{A})^2 \to \exp(-r_s(\mathrm{A}))$ and $1/r_d(\mathrm{A})^2 \to \exp(-r_d(\mathrm{A}))$ are an outcome of the LASSO procedure, not of a directly attempted substitution.

With our 82 materials, the LASSO run takes few seconds (less than 10) for our sets of few thousands candidate features, so the overall selection took less than 5 minutes of CPU time (with MATLAB, on an Intel-i7 CPU).

Our procedure, applied to the above defined set of features, found the following features as best 1D, 2D, and 3D descriptor, already combined linearly with the fitting coefficients in order to approximate the property $\Delta E$ (energies are in eV and radii are in Å).

$$\Delta E = 0.117\frac{\mathrm{EA(B)} - \mathrm{IP(B)}}{r_p(\mathrm{A})^2} - 0.342 \tag{1}$$

$$\Delta E = 0.113\frac{\mathrm{EA(B)} - \mathrm{IP(B)}}{r_p(\mathrm{A})^2} + 1.542\frac{|r_s(\mathrm{A}) - r_p(\mathrm{B})|}{\exp(r_s(\mathrm{A}))} - 0.137 \tag{2}$$

$$\begin{aligned} \Delta E &= 0.108\frac{\mathrm{EA(B)} - \mathrm{IP(B)}}{r_p(\mathrm{A})^2} + 1.790\frac{|r_s(\mathrm{A}) - r_p(\mathrm{B})|}{\exp(r_s(\mathrm{A}))} + \\ &+ 3.766\frac{|r_p(\mathrm{B}) - r_s(\mathrm{B})|}{\exp(r_d(\mathrm{A}))} - 0.0267 \end{aligned} \tag{3}$$

We removed the absolute sign from "IP(B) − EA(B)" as this difference is always negative.

We note the following:

- The stability of fitting the coefficients of the features when the dimensionality is increased is remarkable. This fact gives substance to the idea that the descriptor is built incrementally by adding new dimensions, where the adding a dimension to the descriptor always improves the accuracy of the fit.
- The fact that all selected features belong to class $X$, which is the most populated, is NOT due to the fact that members of the other classes are lost in the large population of class $X$ and "not seen" by LASSO. We have run extensive tests on the classes excluding $X$ and indeed the best-performing descriptors yield RMSE larger than those we have found.
- The stability of the found descriptor was tested by constructing feature spaces where the functional class containing the selected descriptors and other, each time varied, functional classes were included. We always found the above descriptor as the best (resulting in smallest RMSE).
- This final stability check and to some extent also the initial selection procedure as described above can be parallelized, especially if larger amount of data $N >> 82$ is treated, and henceforth much larger $M$ values are achievable according to compressed sensing theory. At present, however, the human time needed for constructing feature spaces was by far larger than the computational time needed for running LASSO, thus no parallelization was implemented.

- A fascinating way to implement the parallel search, which we are presently exploring, is to perform a Monte Carlo (MC) sampling of the sets of features over which LASSO is performed, where the loss function is used as an energy for building the Boltzmann factor for the MC selection rule. Besides, the effective temperature that enters the Boltzmann factor in MC selection rule offers a straightforward way to implement a parallel search in a replica-exchange fashion.
- The description of the iterative procedure for the generation of the feature sets over which LASSO is run gives an idea of the stability of our method, in particular when the direct substitutions $1/r_s(\mathrm{A})^2 \to \exp(-r_s(\mathrm{A}))$ and $1/r_d(\mathrm{A})^2 \to \exp(-r_d(\mathrm{A}))$ was found without giving any information, i.e., any bias, in this direction.
  However, one should realize that even this kind of iteration cannot be pushed too far. With the cumulative dimensionality $M$ of the feature space growing effectively (even though in each constructed feature space this number was kept around few thousands or less), the number of 2D hyperplanes (i.e., the 2D linear fits) grows quadratically with $M$, thus the probability to find one such plane with RMSE almost the same as the previously found best descriptor grows very fast. At that point, several competing pairs could be found and the solution is not anymore unique (even though there is one hyperplane for which the RMSE is the lowest, several others would differ by negligible amounts). Then, one would have a set of possible good 2D descriptors and the choice among them could be dictated by other criteria than RMSE, e.g., in our case, separation between RS and ZB materials, or small MaxAE, where both the latter criteria are not contained explicitly in the RMSE minimization which is performed by LASSO.

## 2. Gaussian-kernel ridge regression with various descriptors

We have performed KRR with several descriptors of various dimensionalities. In each case the optimal $(\lambda, \sigma)$ was sought by running leave-10%-out cross-validation, averaged over 150 random selections of the test/training set.

| ID | Dim. | Description | $\lambda$ | $\sigma$ | RMSE [eV] |
|---|---|---|---|---|---|
| 1 | 1D | our 1D | $3 \cdot 10^{-4}$ | $\sqrt{3000}$ | 0.145 |
| 2 | 2D | $Z_{\mathrm{A}}, Z_{\mathrm{B}}$ | $3 \cdot 10^{-4}$ | 0.1 | 0.191 |
| 3 | 2D | Zunger's $r_\sigma$ and $r_\pi$ [4, 5] | $10^{-5}$ | $\sqrt{10}$ | 0.090 |
| 4 | 2D | our 2D | 0.01 | 10 | 0.102 |
| 5 | 3D | our 3D | $3 \cdot 10^{-3}$ | 10 | 0.082 |
| 6 | 4D | our 4D | $3 \cdot 10^{-3}$ | 10 | 0.062 |
| 7 | 4D | $r_s(\mathrm{A}), r_p(\mathrm{A}), r_s(\mathrm{B}), r_p(\mathrm{B})$ | $3 \cdot 10^{-5}$ | $\sqrt{10}$ | 0.091 |
| 8 | 4D | EA(B), IP(B), $r_p(\mathrm{A}), r_p(\mathrm{B})$ | $10^{-5}$ | $\sqrt{30}$ | 0.095 |
| 9 | 5D | Features building our 2D descriptor [ IP(B), EA(B), $r_s(\mathrm{A}), r_p(\mathrm{A}), r_p(\mathrm{B})$] | $3 \cdot 10^{-5}$ | $\sqrt{10}$ | 0.084 |
| 10 | 6D | $r_s(\mathrm{A}), r_p(\mathrm{A}), r_d(\mathrm{A}), r_s(\mathrm{B}), r_p(\mathrm{B}), r_d(\mathrm{B})$ | $10^{-3}$ | $\sqrt{10}$ | 0.115 |
| 11 | 14D | All atomic features ($A1, A2, A3$) | $3 \cdot 10^{-5}$ | $\sqrt{300}$ | 0.111 |

We make the following observations:

- With several atomic-based descriptors, KRR fits reach levels of RMSE comparable to or slightly better than our linear fit with the LASSO-selected descriptors.
- It is difficult to extract a physical insight out of these several fits. For example, descriptor 7 gives a fit as good as Zunger's descriptor (3), which is made of the same features as 7, but cleverly combined. Furthermore, comparing, e.g., descriptors 7 and 8, it is difficult to understand whether EA and IP of B play a more important role than some atomic radii.
- The performance is not incremental with dimensionality: Descriptor 10 contains the same features as descriptor seven, plus two, intuitively important, features. One thus expects a better

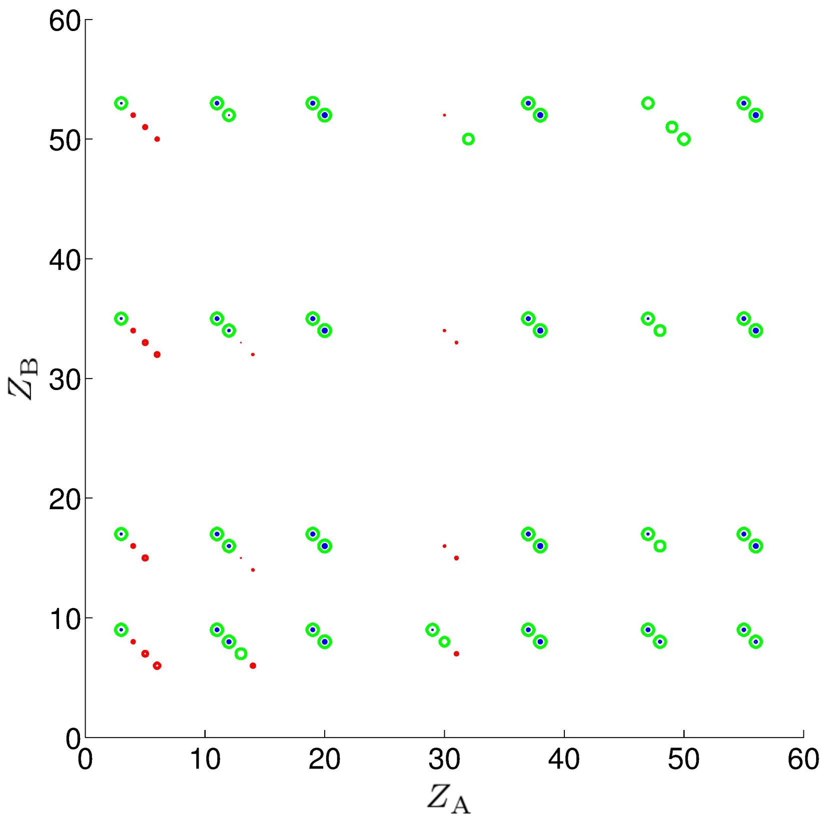


FIGURE 1. KRR fit of $\Delta E(Z_A, Z_B)$ . Green "curves" are for $\Delta E = 0$, blue for $\Delta E = -0.2$ eV, and red for $\Delta E = 0.2$ eV.

performance, which is not the case. The same happens when going to all 14 atomic features (11), where the performance is similar to the 6D descriptor (10), i.e., worse than the 4D (7). Interestingly, the incremental improvement of accuracy with dimensionality is fulfilled by our descriptors.

- By using $Z_A$ and $Z_B$ as descriptors, the RMSE is not particularly large, compared to the baseline at 0.44 eV. However, a look the the level set plot (Fig. 1) reveals that a leave-some-out cross validation may not be enough to spot artifacts. In fact, in Fig. 1, each data point is characterized by a peaked Gaussian (as suggested by the small optimal $\sigma$), i.e., overall it is a completely useless fit.

## 3. A NOTE ON THE LEAVE-10%-OUT CROSS VALIDATION

"Leave-$N$%-out cross validation" and "$N$-fold cross validation" are two similar but different tests performed to assess the stability of a fit. In this paper we have performed (incomplete) "leave-10%-out cross validation" test, i.e., by randomly selecting for 150 times 90% of the materials for the training and the remaining 10% for the prediction. The average errors were clearly converged (within 0.01 eV) after 50 random selections, thus the reported average over 150 samples is a very conservative result. In contrast, in a "10-fold cross validation" the data set is divided in 10 parts and in turn each of the 10 subsets is used for test while the other 9 for training.

## 4. Performance of various descriptor with KRR and linear least square (Extended Table 1 from main text)

| Descriptor<br>$(\lambda,\sigma)$ of KRR | $Z_{\rm A}, Z_{\rm B}$<br>$(3{\cdot}10^{-4}, 0.1)$ | $Z^*_{\rm A}, Z^*_{\rm B}$<br>$(0.01, \sqrt{0.3})$ | $r_\sigma, r_\pi$<br>$(1{\cdot}10^{-5}, \sqrt{10})$ | 1D<br>$(3{\cdot}10^{-4}, \sqrt{3000})$ | 2D<br>$(0.01, 10)$ | 3D<br>$(0.01, 10)$ | 5D<br>$(1{\cdot}10^{-3}, \sqrt{300})$ |
|---|---|---|---|---|---|---|---|
| RMSE | 0.41 $(2{\cdot}10^{-4})$ | 0.40 $(5{\cdot}10^{-3})$ | 0.31 (0.07) | 0.14 (0.14) | 0.10 (0.10) | 0.08 (0.07) | 0.06 (0.06) |
| MAE | 0.28 $(1{\cdot}10^{-4})$ | 0.26 $(3{\cdot}10^{-3})$ | 0.20 (0.05) | 0.12 (0.12) | 0.08 (0.08) | 0.07 (0.06) | 0.05 (0.05) |
| MaxAE | 2.22 $(8{\cdot}10^{-4})$ | 2.19 (0.03) | 1.82 (0.25) | 0.32 (0.31) | 0.32 (0.28) | 0.24 (0.22) | 0.20 (0.19) |
| RMSE, CV | 0.39 (0.19) | 0.21 (0.19) | 0.30 (0.09) | 0.14 (0.15) | 0.11 (0.10) | 0.08 (0.08) | 0.07 (0.07) |
| MAE, CV | 0.29 (0.13) | 0.15 (0.14) | 0.22 (0.07) | 0.12 (0.12) | 0.09 (0.09) | 0.07 (0.06) | 0.05 (0.06) |
| MaxAE, CV | 0.87 (0.43) | 0.45 (0.42) | 0.65 (0.17) | 0.27 (0.27) | 0.18 (0.18) | 0.16 (0.14) | 0.12 (0.13) |

Root mean square error (RMSE), mean absolute error (MAE), and maximum absolute error (MaxAE), in eV, for the least-square fit of all data (first three lines) and for the test set in a leave-10%-out cross validation (CV), averaged over 150 random selections of the training set (last three lines). In parentheses the corresponding errors for Gaussian kernel ridge regression at optimized $(\lambda, \sigma)$. The numbers are reported for selected descriptors, including Zunger's descriptor $(r_\sigma, r_\pi)$ [4]. For $Z^*_{\rm A}$, $Z^*_{\rm B}$, each atom is identified by a string of three random numbers, the errors are averages over 10 random selections.

## 5. Calculated $\Delta E$ of the 82 octet binaries, view of all compounds

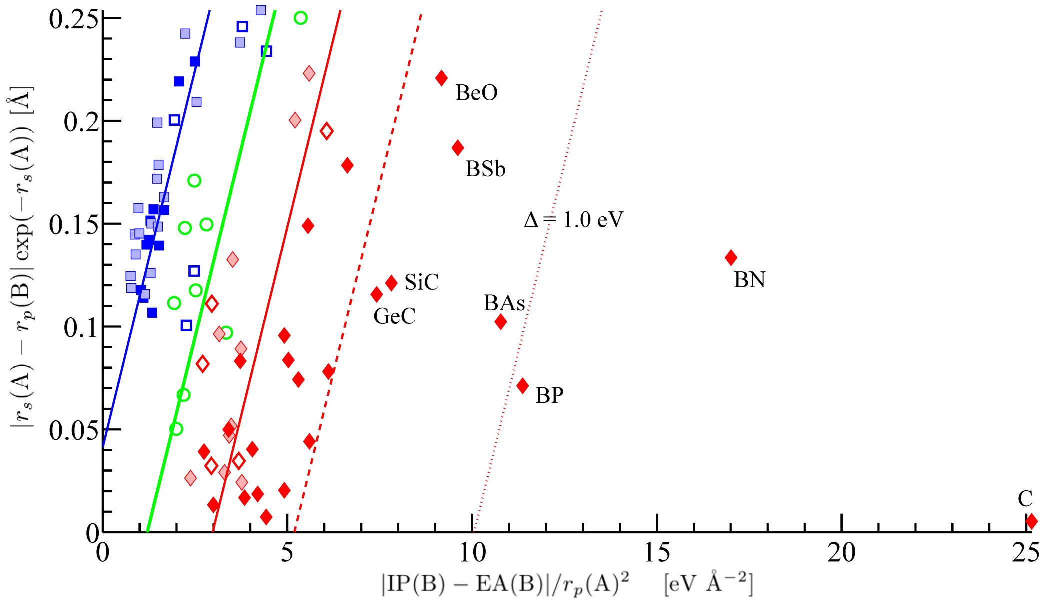


Figure 2. Extended view of Fig.2, bottom, in main text

## 6. Details of the first-principles (DFT) calculations

All DFT calculations are performed with FHI-aims [6], using LDA based on homogeneous electron gas calculations of Ceperley and Alder [7], as parametrized by Perdew and Wang 1992 [8]. All calculations are without spin polarization. The grid settings are *tight* and the basis set is *tier 3*. For both RS and ZB structures, the energy is calculated at the equilibrium lattice constant, which is determined by a 7-point fit to the Birch-Murnaghan equation of state. The scaled ZORA scalar relativistic correction [9] is applied.

## 7. List of the features, used in our model, of the 35 atoms that build the 82 octet binary materials

| $Z_A$ | A | IP [eV] | EA [eV] | EN = $-1/2$(EA+IP) [eV] | Highest occ. KS level [eV] | Lowest unocc. KS level [eV] | $r_s$ [Å] | $r_p$ [Å] | $r_d$ [Å] |
|---|---|---|---|---|---|---|---|---|---|
| 3 | Li | -5.329 | -0.698 | 3.014 | -2.874 | -0.978 | 1.652 | 1.995 | 6.930 |
| 4 | Be | -9.459 | 0.631 | 4.414 | -5.600 | -2.098 | 1.078 | 1.211 | 2.877 |
| 5 | Be | -8.190 | -0.107 | 4.149 | -3.715 | 2.248 | 0.805 | 0.826 | 1.946 |
| 6 | C | -10.852 | -0.872 | 5.862 | -5.416 | 1.992 | 0.644 | 0.630 | 1.631 |
| 7 | N | -13.585 | -1.867 | 7.726 | -7.239 | 3.057 | 0.539 | 0.511 | 1.540 |
| 8 | O | -16.433 | -3.006 | 9.720 | -9.197 | 2.541 | 0.462 | 0.427 | 2.219 |
| 9 | F | -19.404 | -4.273 | 11.839 | -11.294 | 1.251 | 0.406 | 0.371 | 1.428 |
| 11 | Na | -5.223 | -0.716 | 2.969 | -2.819 | -0.718 | 1.715 | 2.597 | 6.566 |
| 12 | Mg | -8.037 | 0.693 | 3.672 | -4.782 | -1.358 | 1.330 | 1.897 | 3.171 |
| 13 | Al | -5.780 | -0.313 | 3.046 | -2.784 | 0.695 | 1.092 | 1.393 | 1.939 |
| 14 | Si | -7.758 | -0.993 | 4.375 | -4.163 | 0.440 | 0.938 | 1.134 | 1.890 |
| 15 | P | -9.751 | -1.920 | 5.835 | -5.596 | 0.183 | 0.826 | 0.966 | 1.771 |
| 16 | Si | -11.795 | -2.845 | 7.320 | -7.106 | 0.642 | 0.742 | 0.847 | 2.366 |
| 17 | Cl | -13.902 | -3.971 | 8.936 | -8.700 | 0.574 | 0.679 | 0.756 | 1.666 |
| 19 | K | -4.433 | -0.621 | 2.527 | -2.426 | -0.697 | 2.128 | 2.443 | 1.785 |
| 20 | Ca | -6.428 | 0.304 | 3.062 | -3.864 | -2.133 | 1.757 | 2.324 | 0.679 |
| 29 | Cu | -8.389 | -1.638 | 5.014 | -4.856 | -0.641 | 1.197 | 1.680 | 2.576 |
| 30 | Zn | -10.136 | 1.081 | 4.527 | -6.217 | -1.194 | 1.099 | 1.547 | 2.254 |
| 31 | Ga | -5.818 | -0.108 | 2.963 | -2.732 | 0.130 | 0.994 | 1.330 | 2.163 |
| 32 | Ge | -7.567 | -0.949 | 4.258 | -4.046 | 2.175 | 0.917 | 1.162 | 2.373 |
| 33 | As | -9.262 | -1.839 | 5.551 | -5.341 | 0.064 | 0.847 | 1.043 | 2.023 |
| 34 | Se | -10.946 | -2.751 | 6.848 | -6.654 | 1.316 | 0.798 | 0.952 | 2.177 |
| 35 | Br | -12.650 | -3.739 | 8.194 | -8.001 | 0.708 | 0.749 | 0.882 | 1.869 |
| 37 | Rb | -4.289 | -0.590 | 2.440 | -2.360 | -0.705 | 2.240 | 3.199 | 1.960 |
| 38 | Sr | -6.032 | 0.343 | 2.844 | -3.641 | -1.379 | 1.911 | 2.548 | 1.204 |
| 47 | Ag | -8.058 | -1.667 | 4.862 | -4.710 | -0.479 | 1.316 | 1.883 | 2.968 |
| 48 | Cd | -9.581 | 0.839 | 4.371 | -5.952 | -1.309 | 1.232 | 1.736 | 2.604 |
| 49 | In | -5.537 | -0.256 | 2.897 | -2.697 | 0.368 | 1.134 | 1.498 | 3.108 |
| 50 | Sn | -7.043 | -1.039 | 4.041 | -3.866 | 0.008 | 1.057 | 1.344 | 2.030 |
| 51 | Sb | -8.468 | -1.847 | 5.158 | -4.991 | 0.105 | 1.001 | 1.232 | 2.065 |
| 52 | Te | -9.867 | -2.666 | 6.266 | -6.109 | 0.099 | 0.945 | 1.141 | 1.827 |
| 53 | I | -11.257 | -3.513 | 7.385 | -7.236 | 0.213 | 0.896 | 1.071 | 1.722 |
| 55 | Cs | -4.006 | -0.570 | 2.288 | -2.220 | -0.548 | 2.464 | 3.164 | 1.974 |
| 56 | Ba | -5.516 | 0.278 | 2.619 | -3.346 | -2.129 | 2.149 | 2.632 | 1.351 |

The table reports the atomic number $Z_A$ of atom A, its Ionization Potential IP and Electron Affinity EA, its Electronegativity EN following Mulliken's definition (this quantity is used to order the AB pair, where EN(A)<EN(B)), the highest occupied and lowest unoccupied Kohns-Sham level, and the radii at which the radial probability density of the valence $s$, $p$, and $d$ orbital are respectively maximal.

## 8. List of the 82 octet binary materials and their LDA and predicted properties

| $Z_A$ | $Z_B$ | A | B | $a_0$(RS) [Å] | $a_0$(ZB) [Å] | $\Delta E$ [eV] | $\Delta E_{1D}$ [eV] | $\Delta E_{2D}$ [eV] | $\Delta E_{3D}$ [eV] | $\boldsymbol{d}_1$ [eV Å$^{-2}$] | $\boldsymbol{d}_2$ [Å] | $\boldsymbol{d}_3$ [Å] | $a_0$(WZ) [Å] | $\Delta E$(WZ) [eV] |
|---|---|---|---|---|---|---|---|---|---|---|---|---|---|---|
| 03 | 09 | Li | F | 3.911 | 4.212 | -0.059 | 0.101 | -0.088 | -0.048 | 3.783 | 0.246 | $2.596 \cdot 10^{-5}$ | 2.978 | 0.011 |
| 03 | 17 | Li | Cl | 4.966 | 5.330 | -0.038 | -0.051 | -0.119 | -0.059 | 2.483 | 0.171 | $3.964 \cdot 10^{-5}$ | 3.769 | 0.005 |
| 03 | 35 | Li | Br | 5.311 | 5.688 | -0.033 | -0.081 | -0.113 | -0.047 | 2.228 | 0.148 | $6.006 \cdot 10^{-5}$ | 4.022 | 0.003 |
| 03 | 53 | Li | I | 5.805 | 6.209 | -0.022 | -0.115 | -0.089 | -0.015 | 1.936 | 0.111 | $6.760 \cdot 10^{-5}$ | 4.390 | 0.002 |
| 04 | 08 | Be | O | 3.584 | 3.762 | 0.430 | 0.733 | 0.560 | 0.569 | 9.171 | 0.221 | $1.063 \cdot 10^{-3}$ | 2.660 | 0.011 |
| 04 | 16 | Be | S | 4.557 | 4.798 | 0.506 | 0.374 | 0.434 | 0.469 | 6.113 | 0.078 | $2.946 \cdot 10^{-3}$ | 3.393 | -0.004 |
| 04 | 34 | Be | Se | 4.834 | 5.084 | 0.495 | 0.314 | 0.428 | 0.465 | 5.597 | 0.044 | $3.783 \cdot 10^{-3}$ | 3.595 | -0.004 |
| 04 | 52 | Be | Te | 5.267 | 5.558 | 0.466 | 0.234 | 0.388 | 0.427 | 4.918 | 0.020 | $4.386 \cdot 10^{-3}$ | 3.930 | -0.004 |
| 05 | 07 | B | N | 3.462 | 3.583 | 1.713 | 1.651 | 1.581 | 1.556 | 17.009 | 0.133 | $2.487 \cdot 10^{-3}$ | 2.534 | -0.014 |
| 05 | 15 | B | P | 4.260 | 4.492 | 1.020 | 0.990 | 1.039 | 0.998 | 11.367 | 0.071 | $8.685 \cdot 10^{-3}$ | 3.177 | -0.008 |
| 05 | 33 | B | As | 4.539 | 4.734 | 0.879 | 0.921 | 0.924 | 0.854 | 10.775 | 0.102 | $1.155 \cdot 10^{-2}$ | 3.347 | -0.006 |
| 06 | 06 | C | C | 3.496 | 3.534 | 2.638 | 2.605 | 2.698 | 2.672 | 25.143 | 0.005 | $1.033 \cdot 10^{-3}$ | 2.499 | -0.024 |
| 11 | 09 | Na | F | 4.504 | 4.965 | -0.146 | -0.080 | -0.257 | -0.209 | 2.238 | 0.242 | $3.721 \cdot 10^{-5}$ | 3.511 | 0.011 |
| 11 | 17 | Na | Cl | 5.465 | 6.031 | -0.133 | -0.170 | -0.235 | -0.170 | 1.469 | 0.172 | $5.681 \cdot 10^{-5}$ | 4.265 | 0.007 |
| 11 | 35 | Na | Br | 5.786 | 6.378 | -0.127 | -0.188 | -0.219 | -0.149 | 1.318 | 0.150 | $8.608 \cdot 10^{-5}$ | 4.510 | 0.005 |
| 11 | 53 | Na | I | 6.260 | 6.892 | -0.115 | -0.208 | -0.186 | -0.108 | 1.146 | 0.116 | $9.689 \cdot 10^{-5}$ | 4.873 | 0.004 |
| 12 | 08 | Mg | O | 4.163 | 4.519 | -0.178 | 0.094 | -0.083 | -0.048 | 3.719 | 0.238 | $7.955 \cdot 10^{-4}$ | 3.196 | 0.030 |
| 12 | 16 | Mg | S | 5.132 | 5.598 | -0.087 | -0.051 | -0.052 | -0.002 | 2.479 | 0.127 | $2.204 \cdot 10^{-3}$ | 3.958 | 0.009 |
| 12 | 34 | Mg | Se | 5.395 | 5.876 | -0.055 | -0.076 | -0.035 | 0.015 | 2.270 | 0.101 | $2.831 \cdot 10^{-3}$ | 4.155 | 0.006 |
| 12 | 52 | Mg | Te | 5.843 | 6.372 | -0.005 | -0.108 | 0.011 | 0.069 | 1.995 | 0.050 | $3.282 \cdot 10^{-3}$ | 4.505 | 0.002 |
| 13 | 07 | Al | N | 4.009 | 4.345 | 0.072 | 0.369 | 0.248 | 0.265 | 6.065 | 0.195 | $2.512 \cdot 10^{-3}$ | 3.069 | 0.025 |
| 13 | 15 | Al | P | 4.998 | 5.436 | 0.219 | 0.133 | 0.259 | 0.259 | 4.053 | 0.040 | $8.773 \cdot 10^{-3}$ | 3.844 | -0.002 |
| 13 | 33 | Al | As | 5.212 | 5.632 | 0.212 | 0.108 | 0.272 | 0.251 | 3.842 | 0.017 | $1.167 \cdot 10^{-2}$ | 3.982 | -0.003 |
| 13 | 51 | Al | Sb | 5.648 | 6.112 | 0.150 | 0.060 | 0.178 | 0.149 | 3.427 | 0.047 | $1.216 \cdot 10^{-2}$ | 4.322 | -0.005 |
| 14 | 06 | Si | C | 4.005 | 4.331 | 0.668 | 0.574 | 0.560 | 0.598 | 7.815 | 0.121 | $7.966 \cdot 10^{-4}$ | 3.063 | 0.003 |
| 14 | 14 | Si | Si | 4.995 | 5.403 | 0.275 | 0.279 | 0.348 | 0.313 | 5.298 | 0.074 | $1.121 \cdot 10^{-2}$ | 3.821 | -0.009 |
| 19 | 09 | K | F | 5.163 | 5.697 | -0.146 | -0.044 | -0.172 | -0.158 | 2.541 | 0.209 | $4.432 \cdot 10^{-3}$ | 4.029 | 0.010 |
| 19 | 17 | K | Cl | 6.078 | 6.773 | -0.165 | -0.147 | -0.199 | -0.194 | 1.668 | 0.163 | $6.767 \cdot 10^{-3}$ | 4.790 | 0.007 |
| 19 | 35 | K | Br | 6.372 | 7.141 | -0.166 | -0.167 | -0.196 | -0.219 | 1.497 | 0.149 | $1.025 \cdot 10^{-2}$ | 5.050 | 0.007 |
| 19 | 53 | K | I | 6.816 | 7.646 | -0.168 | -0.190 | -0.184 | -0.212 | 1.301 | 0.126 | $1.154 \cdot 10^{-2}$ | 5.406 | 0.006 |
| 20 | 08 | Ca | O | 4.710 | 5.121 | -0.266 | -0.050 | -0.207 | -0.244 | 2.495 | 0.229 | $9.595 \cdot 10^{-3}$ | 3.621 | 0.040 |
| 20 | 16 | Ca | S | 5.565 | 6.156 | -0.369 | -0.147 | -0.190 | -0.362 | 1.663 | 0.157 | $2.659 \cdot 10^{-2}$ | 4.353 | 0.024 |
| 20 | 34 | Ca | Se | 5.793 | 6.418 | -0.361 | -0.164 | -0.179 | -0.416 | 1.523 | 0.139 | $3.415 \cdot 10^{-2}$ | 4.538 | 0.020 |
| 20 | 52 | Ca | Te | 6.209 | 6.913 | -0.350 | -0.185 | -0.150 | -0.428 | 1.338 | 0.107 | $3.958 \cdot 10^{-2}$ | 4.888 | 0.014 |
| 29 | 09 | Cu | F | 4.397 | 4.663 | -0.019 | 0.286 | 0.084 | 0.098 | 5.361 | 0.250 | $2.011 \cdot 10^{-3}$ | 3.275 | -0.007 |
| 29 | 17 | Cu | Cl | 4.929 | 5.210 | 0.156 | 0.070 | 0.057 | 0.093 | 3.519 | 0.133 | $3.071 \cdot 10^{-3}$ | 3.684 | 0.000 |
| 29 | 35 | Cu | Br | 5.186 | 5.498 | 0.152 | 0.028 | 0.072 | 0.102 | 3.157 | 0.096 | $4.653 \cdot 10^{-3}$ | 3.890 | -0.001 |
| 29 | 53 | Cu | I | 5.521 | 5.864 | 0.203 | -0.020 | 0.113 | 0.151 | 2.744 | 0.039 | $5.237 \cdot 10^{-3}$ | 4.147 | -0.002 |
| 30 | 08 | Zn | O | 4.212 | 4.493 | 0.102 | 0.313 | 0.151 | 0.169 | 5.589 | 0.223 | $1.996 \cdot 10^{-3}$ | 3.176 | 0.008 |
| 30 | 16 | Zn | S | 4.966 | 5.299 | 0.275 | 0.095 | 0.156 | 0.178 | 3.725 | 0.083 | $5.532 \cdot 10^{-3}$ | 3.747 | -0.002 |
| 30 | 34 | Zn | Se | 5.214 | 5.572 | 0.259 | 0.058 | 0.172 | 0.188 | 3.411 | 0.050 | $7.104 \cdot 10^{-3}$ | 3.940 | -0.004 |
| 30 | 52 | Zn | Te | 5.597 | 5.998 | 0.241 | 0.009 | 0.182 | 0.197 | 2.997 | 0.013 | $8.234 \cdot 10^{-3}$ | 4.241 | -0.005 |
| 31 | 07 | Ga | N | 4.182 | 4.460 | 0.433 | 0.434 | 0.337 | 0.359 | 6.624 | 0.178 | $2.016 \cdot 10^{-3}$ | 3.151 | 0.009 |
| 31 | 15 | Ga | P | 5.049 | 5.395 | 0.341 | 0.177 | 0.352 | 0.372 | 4.427 | 0.007 | $7.040 \cdot 10^{-3}$ | 3.815 | -0.008 |
| 31 | 33 | Ga | As | 5.254 | 5.607 | 0.271 | 0.150 | 0.309 | 0.307 | 4.196 | 0.019 | $9.365 \cdot 10^{-3}$ | 3.965 | -0.011 |
| 31 | 51 | Ga | Sb | 5.645 | 6.052 | 0.158 | 0.097 | 0.149 | 0.132 | 3.743 | 0.089 | $9.758 \cdot 10^{-3}$ | 4.279 | -0.011 |
| 32 | 32 | Ge | Ge | 5.291 | 5.626 | 0.202 | 0.234 | 0.272 | 0.255 | 4.918 | 0.096 | $8.941 \cdot 10^{-3}$ | 3.978 | -0.015 |
| 37 | 09 | Rb | F | 5.464 | 6.012 | -0.136 | -0.169 | -0.276 | -0.250 | 1.478 | 0.199 | $3.739 \cdot 10^{-3}$ | 4.251 | 0.008 |
| 37 | 17 | Rb | Cl | 6.378 | 7.106 | -0.161 | -0.228 | -0.270 | -0.250 | 0.970 | 0.158 | $5.709 \cdot 10^{-3}$ | 5.025 | 0.007 |
| 37 | 35 | Rb | Br | 6.667 | 7.451 | -0.164 | -0.240 | -0.261 | -0.266 | 0.870 | 0.145 | $8.650 \cdot 10^{-3}$ | 5.269 | 0.007 |
| 37 | 53 | Rb | I | 7.104 | 7.977 | -0.169 | -0.253 | -0.243 | -0.253 | 0.756 | 0.125 | $9.736 \cdot 10^{-3}$ | 5.641 | 0.006 |
| 38 | 08 | Sr | O | 5.066 | 5.480 | -0.221 | -0.100 | -0.241 | -0.239 | 2.065 | 0.219 | $5.704 \cdot 10^{-3}$ | 3.875 | 0.035 |
| 38 | 16 | Sr | S | 5.906 | 6.514 | -0.369 | -0.181 | -0.223 | -0.297 | 1.376 | 0.157 | $1.581 \cdot 10^{-2}$ | 4.606 | 0.026 |
| 38 | 34 | Sr | Se | 6.124 | 6.775 | -0.375 | -0.194 | -0.213 | -0.324 | 1.260 | 0.142 | $2.030 \cdot 10^{-2}$ | 4.791 | 0.023 |
| 38 | 52 | Sr | Te | 6.527 | 7.267 | -0.381 | -0.212 | -0.187 | -0.321 | 1.107 | 0.114 | $2.353 \cdot 10^{-2}$ | 5.138 | 0.017 |
| 47 | 09 | Ag | F | 4.791 | 5.202 | -0.156 | 0.160 | -0.044 | -0.020 | 4.281 | 0.254 | $1.362 \cdot 10^{-3}$ | 3.679 | 0.001 |
| 47 | 17 | Ag | Cl | 5.355 | 5.780 | -0.044 | -0.013 | -0.050 | -0.005 | 2.810 | 0.150 | $2.079 \cdot 10^{-3}$ | 4.087 | 0.003 |
| 47 | 35 | Ag | Br | 5.585 | 6.035 | -0.030 | -0.047 | -0.033 | 0.010 | 2.521 | 0.118 | $3.150 \cdot 10^{-3}$ | 4.268 | 0.002 |
| 47 | 53 | Ag | I | 5.897 | 6.355 | 0.037 | -0.085 | 0.008 | 0.059 | 2.191 | 0.067 | $3.546 \cdot 10^{-3}$ | 4.494 | 0.000 |
| 48 | 08 | Cd | O | 4.636 | 4.993 | -0.087 | 0.178 | 0.004 | 0.031 | 4.435 | 0.234 | $1.407 \cdot 10^{-3}$ | 3.531 | 0.011 |
| 48 | 16 | Cd | S | 5.337 | 5.760 | 0.070 | 0.004 | 0.026 | 0.062 | 2.956 | 0.111 | $3.898 \cdot 10^{-3}$ | 4.071 | 0.002 |
| 48 | 34 | Cd | Se | 5.563 | 6.013 | 0.083 | -0.025 | 0.043 | 0.075 | 2.707 | 0.082 | $5.006 \cdot 10^{-3}$ | 4.249 | -0.001 |
| 48 | 52 | Cd | Te | 5.931 | 6.414 | 0.113 | -0.063 | 0.092 | 0.129 | 2.378 | 0.026 | $5.803 \cdot 10^{-3}$ | 4.535 | -0.004 |
| 49 | 07 | In | N | 4.604 | 4.943 | 0.150 | 0.268 | 0.143 | 0.178 | 5.208 | 0.200 | $7.797 \cdot 10^{-4}$ | 3.491 | 0.013 |
| 49 | 15 | In | P | 5.415 | 5.830 | 0.170 | 0.066 | 0.177 | 0.232 | 3.480 | 0.052 | $2.723 \cdot 10^{-3}$ | 4.122 | -0.005 |
| 49 | 33 | In | As | 5.596 | 6.028 | 0.122 | 0.045 | 0.192 | 0.243 | 3.299 | 0.029 | $3.622 \cdot 10^{-3}$ | 4.263 | -0.007 |
| 49 | 51 | In | Sb | 5.976 | 6.454 | 0.080 | 0.003 | 0.146 | 0.198 | 2.943 | 0.032 | $3.774 \cdot 10^{-3}$ | 4.564 | -0.010 |
| 50 | 50 | Sn | Sn | 6.009 | 6.476 | 0.016 | 0.050 | 0.092 | 0.048 | 3.344 | 0.097 | $1.274 \cdot 10^{-2}$ | 4.580 | -0.014 |
| 05 | 51 | B | Sb | 4.931 | 5.186 | 0.581 | 0.784 | 0.662 | 0.577 | 9.612 | 0.187 | $1.204 \cdot 10^{-2}$ | 3.664 | -0.001 |
| 55 | 09 | Cs | F | 5.805 | 6.342 | -0.112 | -0.164 | -0.241 | -0.210 | 1.515 | 0.179 | $3.702 \cdot 10^{-3}$ | 4.487 | 0.006 |
| 55 | 17 | Cs | Cl | 6.730 | 7.485 | -0.152 | -0.225 | -0.248 | -0.226 | 0.995 | 0.145 | $5.652 \cdot 10^{-3}$ | 5.292 | 0.006 |
| 55 | 35 | Cs | Br | 7.021 | 7.829 | -0.158 | -0.237 | -0.244 | -0.245 | 0.892 | 0.135 | $8.564 \cdot 10^{-3}$ | 5.535 | 0.006 |
| 55 | 53 | Cs | I | 7.454 | 8.352 | -0.165 | -0.251 | -0.232 | -0.240 | 0.775 | 0.119 | $9.639 \cdot 10^{-3}$ | 5.904 | 0.005 |
| 56 | 08 | Ba | O | 5.436 | 5.793 | -0.095 | -0.115 | -0.226 | -0.212 | 1.941 | 0.200 | $4.910 \cdot 10^{-3}$ | 4.105 | 0.018 |
| 56 | 16 | Ba | S | 6.271 | 6.866 | -0.326 | -0.190 | -0.224 | -0.276 | 1.294 | 0.151 | $1.361 \cdot 10^{-2}$ | 4.853 | 0.024 |
| 56 | 34 | Ba | Se | 6.475 | 7.128 | -0.350 | -0.203 | -0.218 | -0.302 | 1.185 | 0.140 | $1.747 \cdot 10^{-2}$ | 5.036 | 0.023 |
| 56 | 52 | Ba | Te | 6.862 | 7.614 | -0.381 | -0.220 | -0.200 | -0.305 | 1.041 | 0.118 | $2.025 \cdot 10^{-2}$ | 5.378 | 0.019 |
| 32 | 06 | Ge | C | 4.312 | 4.531 | 0.808 | 0.527 | 0.524 | 0.567 | 7.416 | 0.116 | $4.929 \cdot 10^{-4}$ | 3.202 | 0.000 |
| 50 | 06 | Sn | C | 4.710 | 4.999 | 0.450 | 0.309 | 0.262 | 0.306 | 5.558 | 0.149 | $6.925 \cdot 10^{-4}$ | 3.530 | 0.007 |
| 32 | 14 | Ge | Si | 5.140 | 5.501 | 0.264 | 0.247 | 0.303 | 0.306 | 5.027 | 0.084 | $6.938 \cdot 10^{-3}$ | 3.887 | -0.011 |
| 50 | 14 | Sn | Si | 5.539 | 5.953 | 0.136 | 0.099 | 0.252 | 0.247 | 3.767 | 0.024 | $9.748 \cdot 10^{-3}$ | 4.207 | -0.010 |
| 50 | 32 | Sn | Ge | 5.656 | 6.061 | 0.087 | 0.090 | 0.227 | 0.195 | 3.686 | 0.035 | $1.256 \cdot 10^{-2}$ | 4.283 | -0.013 |

The table reports the atomic number $Z_{\mathrm{A}}$ and $Z_{\mathrm{B}}$ of the binary material AB, the lattice constant $a_0$ for the three considered crystal structures§, the difference in LDA energy between RS ad ZB ($\Delta E = E(\mathrm{RS})$ $-E(\mathrm{ZB})$), the predicted $\Delta E$ for the 1D, 2D, 3D descriptor, the value of the 1D, 2D, and 3D descriptor†, and the difference in energy between ZB and WZ structures ($\Delta E(\mathrm{WZ}) = E(\mathrm{ZB})$ $-E(\mathrm{WZ})$).
All inputs and outputs can be downloaded from on `http://nomad-repository.eu`.

§ For WZ, we have considered the arrangement that is equivalent to ZB up to the first neighbour cell, i.e., with ratio between $c$ and $a$ lattice constants $c/a = \sqrt{8/3}$, and fractional displacement along the $c$ axis of the second atom $u = 3/8$.

† The 1D descriptor is defined by $\boldsymbol{d}_1$, the 2D by the vector $(\boldsymbol{d}_1, \boldsymbol{d}_2)$, the 3D by the vector $(\boldsymbol{d}_1, \boldsymbol{d}_2, \boldsymbol{d}_3)$.

## References

[1] D.L. Donoho. *IEEE Trans. Inform. Theory*, 52:1289, 2006.
[2] E. J. Candés, J. Romberg, and T. Tao. *IEEE Trans. Inform. Theory*, 52:489, 2006.
[3] S. Foucart and H. Rauhut. *A mathematical introduction to compressive sensing.* Springer, New York, 2013.
[4] A. Zunger. *Phys. Rev. B*, 22:5839, 1980.
[5] Y. Saad, D. Gao, T. Ngo, S. Bobbitt, J. R. Chelikowsky, and W. Andreoni. *Phys. Rev. B*, 85:104104, 2012.
[6] V. Blum, R. Gehrke, F. Hanke, P. Havu, V. Havu, X. Ren, K. Reuter, and M. Scheffler. *Comp. Phys. Comm.*, 180:2175, 2009.
[7] D. M. Ceperley and B. J. Alder. *Phys. Rev. Lett.*, 45:566, 1980.
[8] J. P. Perdew and Y. Wang. *Phys. Rev. B*, 45:13244, 1992.
[9] E. van Lenthe, E. J. Baerends, and J. G. Snijders. *J. Chem. Phys.*, 101:9783, 1994.
